# Supplementary material for: Neural Variational Inference and Learning in Undirected Graphical Models
Source: arXiv:1711.02679 source file (2017-11-16)
Supplement: Supplementary file 1 [file appendix.tex]

\section{Recalibration with proper losses}

We now extend our proofs to arbitrary proper losses. In this section, we assume, again, for expository purposes, that calibration is measured using the $\ell_1$ loss. This loss is often considered in the literature; in particular the current best recalibration algorithm by \citet{abernethy11blackwell} targets the $\ell_1$ loss directly.
We will consider general losses in the next section.

\subsection{Notation}

\paragraph{Calibration.}

We define the calibration error of a forecaster $\Fcal$ as
\begin{equation}
C_{T} = \sum_{i=0}^N \left| \rho_T(i/N) - \frac{i}{N} \right| \left( \frac{1}{T} \sum_{t=1}^T \Ind_{\{p_t = \frac{i}{N}\}} \right),
\end{equation}
where $\rho_T(p) = \frac{\sum_{t=1}^T y_t \Ind_{p_t = p}}{\sum_{t=1}^T \Ind_{p_t = p}}$ denotes the frequency at which event $y = 1$ occurred over the times when we predicted $p$.

\begin{defn}
We say that a loss $\ell(y,p) : \{0,1\} \times [0,1] \to \mathbb{R}_+$ is proper if
$p \in \arg\min_q \Exp_{y \sim \text{Ber}(p)} \ell(y, q). $
\end{defn}

Examples of proper losses include the L2 loss $\ell_2(y,p) = (y-p)^2$,
the log-loss $\ell_\text{log}(y,p) = y\log(p) + (1-y)\log(1-p)$,
and the 
the misclassification loss $\ell_\text{mc}(y,p) = (1-y) \Ind_{p < 0.5} + y \Ind_{p \geq 0.5}$ \footnote{There exists a vast literature on proper losses, particularly in connection with calibration. See the extensive survey by Buja et al. (http://www-stat.wharton.upenn.edu/~buja/PAPERS/paper-proper-scoring.pdf) for more details.}. Counter-examples include the L1 and the hinge losses.

\subsection{Calibration implies no internal regret}

Here, we show that a calibrated forecaster also has small internal regret relative to any bounded proper loss.
This lemma is all we need to extend Lemma 2 to general proper losses, i.e. to show that recalibrated forecasts have low regret relative to the uncalibrated forecaster.

Note that the proof used below has the same structure as that of an earlier theorem by Foster and Vohra\footnote{Theorem 1 in Dean Foster and Rakesh Vohra, {\em Calibrated Learning and Correlated Equilibrium}, Games and Economic Behavior, 1997}.

\begin{lemma}
Let $\ell(y,p)$ be a bounded proper loss with $\ell(y,p) < B$ over the entire domain.
Suppose that $\Fcal$ is $(\e, \ell_1)$-calibrated with $C_{T} \leq R_T + \e$ all $T$, 
where $R_T = o(1)$ as $T \to \infty$.
Then w.h.p. $\Fcal$ has a small internal regret with respect to $\ell$:
$$
\intR_{T} = \max_{ij} \sum_{t=1}^T \Ind_{ti} \left( \ell(i/N, y_t)  - \ell(j/N, y_t) \right) \leq 2 B (R_T + \e).
$$
where $\Ind_{ti} = \Ind_{p_t = i/N}$ be the indicator of $\Fcal$ of outputting prediction $i/N$ at time $t$.
%This bound holds uniformly over time $T$.
\end{lemma}

\begin{proof}

Let $T$ be fixed for the rest of this proof.
Let $\Ind_{ti} = \Ind_{p_t = i/N}$ be the indicator of $\Fcal$ outputting prediction $i/N$ at time $t$, let $T_i = \sum_{t=1}^T \Ind_{ti}$ denote the number of time $i/N$ was predicted,  and let
$$ \intR_{T, ij} = \sum_{t=1}^T \Ind_{ti} \left( \ell(i/N, y_t)  - \ell(j/N, y_t) \right) $$
denote the gain (measured using the proper loss $\ell$) from retrospectively switching all the plays of action $i$ to $j$. This value forms the basis of the definition of internal regret (Section 2).

Let $T(i,y) = \sum_{t=1}^T \Ind_{ti} \Ind\{y_t = y\}$ denote the total number of $i/N$ forecasts at times when $y_t = y \in \{0,1\}$. Observe that we have
\begin{align*}
T(i,y) 
& = \sum_{t=1}^T \Ind_{ti} \Ind\{y_t = y\} 
= \frac{\sum_{t=1}^T \Ind_{ti} \Ind\{y_t = y\} }{T_i} T_i
= \frac{\sum_{t=1}^T \Ind_{ti} \Ind\{y_t = y\} }{\sum_{t=1}^T \Ind_{ti}} T_i \\
& = q(i,y) T_i + T_i \left( \frac{\sum_{t=1}^T \Ind_{ti} \Ind\{y_t = y\} }{\sum_{t=1}^T \Ind_{ti}} - q(i,y) \right) \\
& = q(i,y) T_i + T_i \left( \rho_T(i/N) - i/N \right),
\end{align*}
where $q(i,y) = i/N$ if $y=1$ and $1-i/N$ if $y=0$. The last equality follows using some simple algebra after adding and subtracting one inside the parentheses in the second term.

We now use this expression to bound $\intR_{T, ij}$:
\begin{align*}
\intR_{T, ij}
& = \sum_{t=1}^T \Ind_{ti} \left( \ell(i/N, y_t)  - \ell(j/N, y_t) \right) \\
& = \sum_{y \in \{0,1\}} T(i,y) \left( \ell(i/N, y)  - \ell(j/N, y) \right) \\
& \leq \sum_{y \in \{0,1\}} q(i,y) T_i \left( \ell(i/N, y)  - \ell(j/N, y) \right) + \sum_{y \in \{0,1\}} B T_i \left| \rho_T(i/N) - i/N \right| \\
& \leq 2B T_i \left| \rho_T(i/N) - i/N \right|,
\end{align*}
where in the first inequality, we used $\ell(i/N, y)  - \ell(j/N, y) \leq \ell(i/N, y)  \leq B$, and in the second inequality we used the fact that $\ell$ is a proper loss.

Since internal regret equals $\intR_{T} = \max_{i,j} \intR_{T, ij}$, we have
\begin{align*}
\intR_{T}
& \leq \sum_{i=1}^N \max_{j} \intR_{T, ij} 
 \leq 2B \sum_{i=0}^N T_i \left| \rho(i/N) - i/N \right| 
 \leq 2 B ( R_T + \e ).
\end{align*}

\end{proof}

\subsection{Recalibrated forecasts have low regret relative to uncalibrated forecasts}

We now use the above result to prove an extension of Lemma 2 to general proper losses, i.e. we show that the forecasts recalibrated using Algorithm 2 have low regret relative to the baseline uncalibrated forecasts.

\begin{lemma}\label{lem:regret}
Consider an instance of Algorithm 2 with
parameters $M \geq N$, and $\ell$ be a proper loss that is
\begin{enumerate}
\item Bounded in absolute value by $B>0$
\item $\ell(y_t, p) \leq \ell(y_t, j/M) + B/M$ whenever $p \in [j/M, (j+1)/M)$.
\item $\ell(y_t, p) \leq \ell(y_t, i/N) + B/N$ whenever $p \in [i/N, (i+1)/N)$.
\end{enumerate}
The recalibrated forecasts $p_t$ have vanishing $\ell$-loss regret relative to $\palg_t$:
$$ \lim_{T\to\infty} \left( \frac{1}{T} \sum_{t=1}^T \ell (y_t , p_t) - \frac{1}{T} \sum_{t=1}^T \ell(y_t , \palg_t) \right) < 3B/N. $$
\end{lemma}

\begin{proof}
By the previous lemma, we know that an algorithm with resolution $\frac{1}{N}$ whose calibration error is bounded by $R_T = o(1)$ also minimizes internal regret at a rate of $2BR_T$, and thus external regret at a rate of $2NBR_T$.

Next, let us use $\Ind_{j,t} = \Ind \{\palg_t \in [\frac{j-1}{M},\frac{j}{M})\}$ to indicate that $\Fcal_j$ was called at time $t$. Also, let $i_j$ denote the index $i \in [N]$ associated with the interval $[i/N, (i+1)/N)$ in which $j/M$ falls.

We establish our main claim as follows:
\begin{align*}
& \frac{1}{T} \sum_{t=1}^T  \ell (y_t , p_t) - \frac{1}{T} \sum_{t=1}^T \ell (y_t , \palg_t) \\
& \;\; = \frac{1}{T} \sum_{t=1}^T \left( \sum_{j=1}^M \left( \ell (y_t , p_t) - \ell (y_t , \palg_t) \right) \Ind_{j,t} \right) \\
& \;\; < \frac{1}{T} \sum_{t=1}^T \left( \sum_{j=1}^M \left( \ell (y_t , p_t) - \ell (y_t , \frac{j}{M}) \right) \Ind_{j,t} + \frac{B}{N}\right) \\
& \;\; < \frac{1}{T} \sum_{t=1}^T \left( \sum_{j=1}^M \left( \ell (y_t , p_t) - \ell (y_t , \frac{i_j}{N}) \right) \Ind_{j,t} + \frac{2B}{N}\right) \\
& \;\; \leq N B \sum_{t=1}^T \sum_{j=1}^M \frac{T_j}{T} R_{T_j} + \frac{3B}{N},
\end{align*}
where $R_{T_j}$ is a bound on the calibration error of $\Fcal_j$ after $T_j$ plays. 

%The first inequality holds because $|\palg_t - \frac{j}{M}| \leq \frac{1}{M} \leq \frac{1}{N}$ when $\Ind_{j,t} = 1$ and because $\ell_2(\palg_t, y_t) \geq \ell_2(\frac{j}{M},y_t) + \frac{\partial \ell_2}{\partial p}(p,y_t)(\frac{j}{M}-\palg_t)$. 
In the first two inequalities, we use our assumption on the loss $\ell$, and that $ \frac{1}{M} \leq \frac{1}{N}$.
%Note that this bound holds for other convex loss functions.
%We repeat the same argument in the second inequality using the fact that $|\frac{i_j}{N} - \frac{j}{M}| \leq \frac{1}{N}$ for some $i_j$.
The last inequality follows because $\Fcal_j$ minimizes external regret w.r.t.~the constant action $i_j$ at a rate of $NBR_{T_j}$.
\end{proof}

\subsection{Correctness of Algorithm 2 using general proper losses}

We now prove our main result about the correctness of Algorithm 2. 

\begin{lemma}
Let $\ell$ be a proper loss that is
\begin{enumerate}
\item Bounded in absolute value by $B\geq 1$
\item $\ell(y_t, p) \leq \ell(y_t, j/M) + B/M$ whenever $p \in [j/M, (j+1)/M)$.
\item $\ell(y_t, p) \leq \ell(y_t, i/N) + B/N$ whenever $p \in [i/N, (i+1)/N)$.
\end{enumerate}
Let $\Fcal$ be an $(\ell_1, \epsilon/3B)$-calibrated online algorithm with resolution $N \geq 3B/\epsilon$. 
Then Algorithm 2 is an $\epsilon$-accurate online recalibration algorithm for the loss $\ell$.
%Let $\Fcal$ be an $\e$-calibrated online algorithm with resolution $N$. Then \algorithmref{recal} with parameters $\Fcal$ and $4N$ is an $\e$-accurate online recalibration algorithm for the $\ell_2$ loss.
\end{lemma}

\begin{proof}
It is easy to show that Algorithm 2 is $(\ell_1, \e/3B)$-calibrated by the same argument as Lemma 1 (see the next section for a formal proof). By Lemma 4, its regret w.r.t. the raw $\palg_t$ tends to $< 3B/N < \e$. Hence, the theorem follows.
\end{proof}

Finally, we would like to instantiate this lemma with the misclassification loss
$\ell_\text{mc}(y,p) = (1-y) \Ind_{p < 0.5} + y \Ind_{p \geq 0.5}$, which is arguably the most interesting and general loss.

\begin{theorem}
Let $\Fcal$ be an $(\ell_1, \epsilon/3)$-calibrated online algorithm with resolution $N \geq 3/\epsilon$, where $N$ is a power of two. 
Then Algorithm 2 is an $\epsilon$-accurate online recalibration algorithm for the loss $\ell_\text{mc}$.
\end{theorem}

\begin{proof}
We only need to show that $\ell_\text{mc}$ satisfies the requirements of the above lemma. Clearly, we have $B=1$. Note that if $N$ is a power of two, the point $0.5$ is contained in an interval $[0.5, 0.5+1/N)$; hence, by construction, $\ell_\text{mc}(y,p)$ satisfies the other two conditions, since changing $p$ doesn't affect the loss, as long as $p$ is in the same interval.
\end{proof}

\section{Calibration using general losses}

In the previous section, we assumed that we defined calibration using the $\ell_1$ loss; here, we argue that any convex loss $\ell$ may be used, although this may affect the convergence rate of our method. We give a detailed analysis of convergence rates for the $\ell_2$ loss.

\subsection{Notation}

We define the calibration error relative to loss $\ell$ as
\begin{equation}
C_{T, \ell} = \sum_{i=0}^N \ell \left( \rho_T(i/N), \frac{i}{N} \right) \left( \frac{1}{T} \sum_{t=1}^T \Ind_{\{p_t = \frac{i}{N}\}} \right),\label{eqn:cal_loss}
\end{equation}
which is the weighted distance between the $\rho_T(i/N)$ and the predicted probabilities $\frac{i}{N}$.

\begin{defn}[Abernethy et al. (2011)]
We say that $\Fcal$ is an $(\ell, \e)$-calibrated algorithm with resolution $1/N$ if 
$$ \lim \sup_{T \to \infty} C_{T, \ell} \leq \e. $$
%We say $\Fcal$ is well-calibrated if it is $\e$-calibrated for all $\e > 0$.
\end{defn}

Abernethy et al. (2011) gave examples of $(\ell_1, \e)$-calibrated algorithms, where $\ell_1(x,y) = |x-y|$ denotes the L1 norm. Since L1 is the largest norm, their algorithm extends directly to other losses, e.g. $\ell_p(x,y) = ||x-y||_p^p$.

\subsection{Analysis}

\paragraph{Arbitrary convex losses $\ell$.}

First, it is not hard to see that if $C_{T,\ell} \to 0$ for some convex, continuous $\ell$, then it must be the case that $C_{T,\ell_1} \to 0$ as well. This can be established using a simple real analysis style argument based on continuity. 

More generally, since we can make $C_{T,\ell} < \e$ for an arbitrarily small $\e >0$ by increasing $N$ and $T$, this means that we can make $C_{T,\ell}$ arbitrarily small as well. The only question has to do with the rate of convergence, and this varies depending on the loss.

\paragraph{An analysis for the $\ell_2$ loss.}

We can easily derive the correct convergence late in simple cases, such as for the $\ell_2$ loss. It follows form the bound $||x||_1 \leq \sqrt{d} ||x|_2$ that
$$\sum_{i=0}^N w_i |a_i| \leq \sum_{i=0}^N \sqrt{w_i} |a_i| \leq \sqrt{N+1} \sqrt{\sum_{i=0}^N w_i a_i^2} , $$
where we assume that $0 \leq w_i \leq 1$. Using this with our definition of calibration, we find that
$$
\sum_{i=0}^N \left| \rho_T(i/N) - \frac{i}{N} \right| \left( \frac{1}{T} \sum_{t=1}^T \Ind_{\{p_t = \frac{i}{N}\}} \right) \leq \sqrt{N+1}\left(\sqrt{R_T} + \sqrt{e}\right)
$$
when $C_{T, \ell_2} \leq R_T + \e$. This means that if an algorithm minimizes L2 calibration, the L1 calibration term will converge more slowly to a larger value. To achieve a level of accuracy we need to (among other things) square the resolution parameter $N$.

%\subsection{Online recalibration}
%
%\begin{defn}
%We say that $A$ is an $(\e, \ell_\textrm{cal}, \ell_\textrm{reg})$-accurate online recalibration algorithm if
%\begin{itemize}
%\item The forecasts $p_t = A(\palg_t)$ are $(\e, \ell_\textrm{cal})$-calibrated.
%\item The $\ell_\textrm{reg}$ regret of $p_t$ with respect to $\palg_t$ is small:  
%$$\lim_{T \to \infty} \frac{1}{T} \sum_{t=1}^T \left( \ell_\textrm{reg}(p_t , y_t) - \ell_\textrm{reg}(\palg_t , y_t)\right) \leq \epsilon.$$
%\end{itemize}
%\end{defn}

\subsection{Proving that calibration holds under any loss}

Finally, we give a simple extension of Lemma 1, that shows that Algorithm 2 preserves the $(\ell, \e)$-calibration of its input forecaster. We use the same notation as in the main paper, except that we add a $\ell$ subscript to denote the loss.

\begin{lemma}\label{lem:calibration}
If each $\Fcal_j$ is $(\e, \ell)$-calibrated with convex loss $\ell$ and with
$ C^{(j)}_{T, \ell} \leq R_{T_j} + \e $
for all $T$,
where $R_{T_j} = o(1)$ as $T_j \to \infty$, then Algorithm 2 is also $(\e, \ell)$-calibrated and
\begin{align}
C_{T, \ell} \leq \sum_{j=1}^M \frac{T_j}{T} R_{T_j} + \e. \label{eqn:rate}
\end{align}
This bound holds uniformly over time $T$.
%where $T_j$ is the number of plays of $\Fcal_j$ at time $T$.
%$$C_T \leq R_T + \e.$$
\end{lemma}
\begin{proof}
Let $\wsupj_i = \sum_{t=1}^T \wsupj_{t,i}$. We may write
\begin{align*}
  C_{T,i} 
& = \frac{\sum_{t=1}^T \Ind_{t,i}}{T} \ell \left(  \rho_T(i/N) , \frac{i}{N} \right) \\
& = \frac{\sum_{j=1}^M \sum_{t=1}^T \wsupj_{t,i}}{T} \ell \left( \frac{\sum_{j=1}^M \sum_{t=1}^T \wsupj_{t,i} y_t}{\sum_{j=1}^M \sum_{t=1}^T \wsupj_{t,i}}  , \frac{i}{N} \right) \\
& = \frac{\sum_{j=1}^M \wsupj_i}{T} \ell \left( \frac{\sum_{j=1}^M \wsupj_i \rjt(i/N) }{\sum_{j=1}^M \wsupj_i }  , \frac{i}{N} \right) \\
& \leq \sum_{j=1}^M \frac{\wsupj_i}{T} \ell \left( \rjt(i/N), \frac{i}{N} \right) = \sum_{j=1}^M  \frac{T_j}{T} C^{(j)}_{T, i, \ell},
\end{align*}
where in the last line we used Jensen's inequality. 
Plugging in this bound in the definition of $C_{T, \ell}$, we find that 
%$ C_T = \sum_{i=1}^N  C_{T,i} \leq \sum_{j=1}^M \sum_{i=1}^N \frac{T_j}{T} C^{(j)}_{T,i} $ which in turn can be bounded as
%\begin{align}
% C_T \leq \sum_{j=1}^M \frac{T_j}{T} R_{T_j} + \e. \label{eqn:rate}
%\end{align}
\begin{align}
 C_{T, \ell}
& = \sum_{i=1}^N  C_{T,i, \ell}
\leq \sum_{j=1}^M \sum_{i=1}^N \frac{T_j}{T} C^{(j)}_{T,i, \ell} \nonumber\\
& \leq \sum_{j=1}^M \frac{T_j}{T} R_{T_j} + \e, \nonumber
\end{align}
Since each $R_{T_j} \to 0$, Algorithm 2 will be $\e$-calibrated.
\end{proof}

Note that this proof is essentially identical to that of the main paper.
